# Supplementary material for: PAC Prediction Sets Under Covariate Shift
Source: arXiv:2106.09848 source file (2022-03-16)
Supplement: Supplementary file 1 [file appendix_old.tex]

%% !TEX root = ../pac_ps_cov.tex

\clearpage
%%
%%
%%
\section{Proof of Theorem \ref{thm:cp_bound}} \label{apdx:cp_bound_proof}

%% theorem
\begin{theorem}%[Application of Clopper-Pearson] 
\label{thm:cp_bound}
We have $\Prob_{S_m\sim P^m}[L_P(C)\le U_{\text{CP}}(C,S_m,\delta)]\ge1-\delta$, where 
\begin{align*}
U_{\text{CP}}(C,S_m,\delta)\coloneqq\overline{\theta}(\bar{L}_{S_m}(C);m,\delta).
\end{align*}
%For any $\Ch \in \Ts$, $\delta \in [0, 1]$, $m \in \naturalnum \cup \{0\}$, and $P$, the following holds with probability at least $1 - \delta$:
%\eqa{
%	L_P(\Ch) \leq \underbrace{ \inf  \left\{ \theta \in [0, 1] \vmid \Prob_{Z_\theta} \[ Z_\theta \leq \sum_{i=1}^m \mathbbm{1} \( y_i \notin \Ch(x_i) \) \] \leq \delta \right\} \cup \Big\{1\Big\} }_{ U_{\text{CP}}(\Ch, S_m, \delta)} , \label{eq:ucb_cp}
%}
%where $Z_\theta \sim \text{Bino}(m, \theta)$ and $S_m \sim P^m$.
%\eqa{
%	L_P(\Ch) \leq \underbrace{\inf  \left\{ \theta \in [0, 1] \vmid F(\bar{L}_{S_m}(\Ch); m, \theta) \leq \delta \right\} \cup \Big\{1\Big\}}_{ \eqqcolon U_{\text{CP}}(\Lb_{S_m}(\Ch), \delta)}, \label{eq:ucb_cp}
%}
%where $F$ is the CDF of $\text{Bino}(m, \theta)$ and $S_m \sim P^m$.
\end{theorem}

The population loss $L_P(C)$ is the success probability parameter of the Binomial distribution with $m$ trials followed by the nun-normalized empirical risk. Thus, finding an upper confidence bound for $L_P(C)$ is equivalent to the upper Clopper-Pearson interval, which states \citep{clopper1934use,cai2005one}:
%\eqas{
%	\Prob_{S_p} \[ p \le \inf \Big\{ \theta \;\Big|\; \Prob_{S_\theta}\[ S_\theta \le S_p \] \le \delta \Big\} \cup \Big\{ 1 \Big\} \] \ge 1 - \delta,
%}
\eqas{
	\Prob_{K} \[ p \le \inf \Big\{ \theta \;\Big|\; F(K; m, \theta) \le \delta \Big\} \cup \Big\{ 1 \Big\} \] \ge 1 - \delta,
}
where $p$ is the success probability, $K$ is the observed number of successes, where $K \sim \text{Bino}\(m, p \)$, $F$ is the CDF of the binomial distribution $\text{Bino}(m, \theta)$, and $1 - \delta$ is the confidence level. 
Considering $L_P(C)$ is the success probability and $\bar{L}_{S_m}(C)$ as the observed number of successes, we have $\bar{L}_{S_m}(C) \sim \text{Bino}(m, L_P(C))$, so the following also holds:
\eqas{
	\Prob_{S_m} \[ L_P(C) \le \inf \Big\{ \theta \;\Big|\; F(\bar{L}_{S_m}(C); m, \theta) \le \delta \Big\} \cup \Big\{ 1 \Big\} \] \ge 1 - \delta,
}
as claimed.


%%
%%
%%
\section{Proof of Lemma \ref{lem:mono_CP}} \label{apdx:mono_CP_proof}
%\textbf{Monotonicity in $m$.} 
Recall that $F(k; m, \theta)$ is the cumulative distribution function of a binomial distribution $\text{Binom}\(m, \theta\)$, or equivalently of the random variable $\sum_{i=1}^{m} X_{i}$, where $X_i \sim \text{Bernoulli}(\theta)$ are i.i.d.

%% the decreasing case
\textbf{Decreasing case.}
If $\Lb_{S_{m-1}}(C) = \Lb_{S_{m}}(C) = k$, $k \le m-1$; then 
%we have
%\eqas{
%	F(k; m, \theta) 
%	&\coloneqq \Prob\[ \sum_{i=1}^m X_{i} \le k \] \\
%	&= \Prob\[ \( \sum_{i=1}^m X_{i} \le k \) \wedge \( X_{m} = 0 \vee X_{m} = 1 \)\] \\
%	&= \Prob\[ \sum_{i=1}^m X_{i} \le k  \vmid X_{m} = 0 \] \Prob\[ X_{m} = 0 \]  + \Prob\[ \sum_{i=1}^m X_{i} \le k  \vmid X_{m} = 1 \] \Prob\[ X_{m} = 1 \] \\
%	&= \Prob\[ \sum_{i=1}^m X_{i} \le k  \vmid X_{m} = 0 \] (1 - \theta) + \Prob\[ \sum_{i=1}^m X_{i} \le k  \vmid X_{m} = 1 \] \theta \\
%	&= \Prob\[ \sum_{i=1}^{m-1} X_{i} \le k \] (1 - \theta) + \Prob\[ \sum_{i=1}^{m-1} X_{i} \le k - 1 \] \theta \\
%	&= F(k; m-1, \theta)(1 - \theta) + F(k-1; m-1, \theta) \theta \\
%	&= F(k; m-1, \theta) - \theta \( F(k; m-1, \theta) + F(k-1; m-1, \theta) \) \\
%	&\le F(k; m-1, \theta),
%}
%which implies that $F$ is monotonically decreasing in $m$.
we have
$$
\sum_{i=1}^m X_{i} \le k \Rightarrow
\sum_{i=1}^{m-1} X_{i} \le k,
$$
hence
$$
\Prob\[ \sum_{i=1}^m X_{i} \le k \]\subseteq
\Prob\[ \sum_{i=1}^{m-1} X_{i} \le k\],
$$
so $F(k; m, \theta) \le F(k; m-1, \theta)$.

Then, 
we have
\eqas{
U_{\text{CP}}(\Lb_{S_m}(C), \delta) 
% &\coloneqq \inf  \left\{ \theta \in [0, 1] \vmid \Prob_{Z_\theta} \[ Z_\theta \leq k \] \leq \delta \right\} \cup \{1\} \\
&\coloneqq \inf \left\{ \theta \in [0, 1] \vmid  F(k; m, \theta) \leq \delta \right\} \cup \{1\} \\
&\le \inf \left\{ \theta \in [0, 1] \vmid  F(k; m-1, \theta) \leq \delta \right\} \cup \{1\} \\
&\eqqcolon  U_{\text{CP}}(\Lb_{S_{m-1}}(C), \delta), 
}
thus $U_{\text{CP}}$ is monotonically decreasing (or rather, non-increasing) in $m$.

%% increasing case
\textbf{Increasing case.}
If $\Lb_{S_{m-1}}(C) + 1 = \Lb_{S_{m}}(C) = k$, 
%similarly we have
%\eqas{
%	F(k; m, \theta) 
%	&= F(k; m-1, \theta)(1 - \theta) + F(k-1; m-1, \theta) \theta \\
%	&= F(k; m-1, \theta)(1 - \theta) + F(k-1; m-1, \theta) (1 - 1 + \theta) \\
%	&= F(k-1; m-1, \theta) + (1-\theta) (F(k; m-1, \theta) - F(k-1; m-1, \theta)) \\
%	&\ge F(k-1; m-1, \theta)
%}
%which implies that $F$ is monotonically increasing in $(m, k)$ jointly. 
we have
$$
\sum_{i=1}^{m-1} X_{i} \le k-1 \Rightarrow
\sum_{i=1}^{m} X_{i} \le k,
$$
hence
$$
\Prob\[ \sum_{i=1}^{m-1} X_{i} \le k-1 \]\subseteq
\Prob\[ \sum_{i=1}^{m} X_{i} \le k\],
$$
so $F(k-1; m-1, \theta) \le F(k; m, \theta)$.

Then, we have
\eqas{
 U_{\text{CP}}(\Lb_{S_m}(C), \delta) 
% &\coloneqq \inf  \left\{ \theta \in [0, 1] \vmid \Prob_{Z_\theta} \[ Z_\theta \leq k \] \leq \delta \right\} \cup \{1\} \\
 &\coloneqq \inf \left\{ \theta \in [0, 1] \vmid  F(k; m, \theta) \leq \delta \right\} \cup \{1\} \\
 &\ge \inf \left\{ \theta \in [0, 1] \vmid  F(k-1; m-1, \theta) \leq \delta \right\} \cup \{1\} \\
 &\eqqcolon  U_{\text{CP}}(\Lb_{S_{m-1}}(C), \delta), 
}
thus $U_{\text{CP}}$ is monotonically  jointly increasing (or rather, non-decreasing) in $(m, \Lb_{S_{m}}(C))$.



%%
%%
%%
\section{Proof of Theorem \ref{thm:rscp_bound}} \label{apdx:rscp_bound_proof}

\begin{theorem} \label{thm:rscp_bound}
%For any $\Ch \in \Ts$, $\delta \in [0, 1]$, $m \in \naturalnum \cup \{0\}$, $P$, $Q$, and $w^*$, the following holds with probability at least $1 - \delta$:
We have $\Prob_{S_m\sim P^m,V\sim U^m}\left[L_Q(C) \le U_{\text{RSCP}}(C, S_m, V, b, w, \delta)\right]\ge1-\delta$, where
\eqa{
U_{\text{RSCP}}(C, S_m, V, w, b, \delta) \coloneqq U_{\text{CP}}(C,T_n(S_m,V,w,b),\delta).
%\leq \underbrace{\inf  \left\{ \theta \in [0, 1] \vmid F( \Lb_{S_m, V}(\Ch); \mathbf{1}^T \sigma, \theta) \leq \delta \right\} \cup \Big\{1\Big\}}_{\coloneqq U_{\text{RSCP}}(\Ch, S_m, V, w, \delta)},
\label{eq:ucb_cp_rejection}
}
%$V \sim \text{Unif}(0, 1)^m$, 
%$S_m \sim P^m$,
%$\sigma_i \coloneqq \mathbbm{1}(V_i \le w^*(x_i)/\max_{x \in \Xs} w^*(x))$ for $i \in [m]$,
%$F$ is the CDF of $\text{Bino}( \mathbf{1}^T \sigma, \theta)$,  and
%$\smash{\Lb_{S_m, V}(\Ch) \coloneqq \sum_{i=1}^m \sigma_i \mathbbm{1}( y_i \notin \Ch(x_i) )}$.
%where $S_\theta \sim \text{Bino}(N, \theta)$,
%$N \sim \text{Bino}(m, \frac{1}{b})$, 
%and
%$\sigma_i \sim \text{Bern}(\frac{w(x_i)}{b})$.
\end{theorem}

The rejection sampling prediction set consists of two steps: 1) generate target samples, using source samples $S_m$, importance weights $w$, and an upper bound on their maximum value $b$, and 2) construct the Clopper-Pearson prediction set using the generated target samples.

%% rejection sampling part
From rejection sampling, we choose $N \coloneqq \sum_{i=1}^m \sigma_i$ samples from $S_m$, denoting them by $T_N$; here, $N \sim \text{Bino}\(m, \frac{1}{b}\)$, and $\frac{1}{b}$ is the acceptance probability \citep{vonNeumann1951}---\ie
\eqas{
	\Prob\[ V \le \frac{w(X)}{b} \] = \frac{1}{b}.
}
The samples in $T_N$ are independent and identically distributed, conditionally on the random number $N$ of samples being equal to any fixed value $n$. The reason is that one can view the rejection sampling algorithm proceeding in stages, iterating through the samples one by one. The first stage starts at the very beginning, and then each stage ends when a datapoint is accepted, followed by starting a new stage at the next datapoint. The last stage ends at the last datapoint. 

Based only on the source samples observed in one stage, rejection sampling produces a sample from the target distribution. Thus, within each stage, we produce one sample from the target distribution, and because each stage is independent of all the other ones, conditionally on any number of stages reached, our produced target samples are iid.  Thus, we can use the Clopper-Pearson bound conditionally on each $N=n$.

%% our bound
Given $T_N$, we construct the prediction set based on the i.i.d. assumption. Denoting the CP bound by $U_\text{CP}(C, T_N, \delta)$% \ee{$Z_n$ vs $T_N$?}, where $Z_n$ are the $n$ labeled examples
, it follows that
\eqas{
\Prob_{N, T_N} \[ L_Q(C) \leq U_{\text{CP}}(C, T_N, \delta) \]
&= \sum_{n=0}^{m} \Prob_{T_n} \[ L_Q(C) \leq U_{\text{CP}}(C, T_n, \delta) \] \Prob\[ N =n \] \\
&\ge \sum_{n=0}^{m} (1 - \delta) \Prob\[ N =n \] \\
&= 1 - \delta,
}
as claimed.


%{\color{red}
%Recall that 
%\eqas{
%\sigma_i &\coloneqq \mathbbm{1} \( V_i \le \frac{w^*(x_i)}{\max_{x \in \Xs} w^*(x)} \) \text{~for~} i \in \{1, \dots, m \}, \\
%\Lb_{S_m, V}(\Ch) &\coloneqq \sum_{i=1}^m \sigma_i \mathbbm{1}( y_i \notin \Ch(x_i) ), \text{~and} \\
%\bar{L}_{S_m}(\Ch) &\coloneqq \sum_{(x, y) \in S_m} \mathbbm{1}\( y \notin \Ch(x) \) \\
%\bar{L}_{T_n}(\Ch) &\coloneqq \sum_{(x, y) \in T_n} \mathbbm{1}\( y \notin \Ch(x) \).
%}
%Let $U_{\text{RSCP}}' \coloneqq U_{\text{RSCP}}(\Ch, S_m, V, w, \delta)$ and
%$T_n \coloneqq \{(x_i, y_i) \in S_m \mid \sigma_i = 1\} \subseteq S_m$; thus 
%$n \coloneqq \mathbf{1}^T \sigma$, and
%$\bar{L}_{S_m, V}(\Ch) = \bar{L}_{T_n}(\Ch)$. Then, we have
%\eqas{
%& \Prob_{S_m, V}\[ L_Q(\Ch) \le U_{\text{RSCP}}' \] \\
%&= \int_0^1 \Prob_{S_m}\[ L_Q(\Ch) \le U_{\text{RSCP}}' \vmid V=v \] \Prob_{V}\[ V = v \] \mathrm{d} v \\
%&= \int_0^1 \Prob_{S_m}\[ L_Q(\Ch) \le U_{\text{RSCP}}' \vmid V=v \] \mathrm{d} v \\
%&= \int_0^1 \Prob_{S_m}\[ L_Q(\Ch) \le \inf  \left\{ \theta \in [0, 1] \vmid F( \Lb_{S_m, v}(\Ch); \mathbf{1}^T \sigma, \theta) \leq \delta \right\} \cup \Big\{1\Big\} \] \mathrm{d} v \\
%&= \int_0^1 \Prob_{S_m}\[ L_Q(\Ch) \le \inf  \left\{ \theta \in [0, 1] \vmid F( \Lb_{S_m, v}(\Ch); n, \theta) \leq \delta \right\} \cup \Big\{1\Big\} \] \mathrm{d} v \\
%&= \int_0^1 \Prob_{S_m}\[ L_Q(\Ch) \le \inf  \left\{ \theta \in [0, 1] \vmid F( \Lb_{T_n}(\Ch); n, \theta) \leq \delta \right\} \cup \Big\{1\Big\} \] \mathrm{d} v \\
%&= \int_0^1 \Prob_{T_n}\[ L_Q(\Ch) \le \inf  \left\{ \theta \in [0, 1] \vmid F( \Lb_{T_n}(\Ch); n, \theta) \leq \delta \right\} \cup \Big\{1\Big\} \] \mathrm{d} v \\
%&= \int_0^1 \Prob_{T_n}\[ L_Q(\Ch) \le U_{\text{CP}}(\bar{L}_{T_n}(\Ch), \delta)  \] \mathrm{d} v \\
%&\ge \int_0^1 1 - \delta  \mathrm{d} v \\
%&= 1 - \delta,
%}
%as claimed.
%\SPI{is it rigorous?}
%}


%%
%%
%%
\section{Proof of Theorem \ref{thm:e2e_ps_bound}} \label{apdx:e2e_ps_bound_proof}

%\begin{theorem}\label{thm:e2e_ps_bound}
%For any $\smash{\Ch \in \Ts}$, $w^*$, $\delta_C, \delta_w \in (0, 1)$, $m, n \in \naturalnum \cup \{0\}$, $P$, and $Q$, if
%\eqas{
%	\Probop_{S_m^X, T_n^X}\Big[w^* \in \Ws(S_m^X, T_n^X, \delta_{w})\Big] \ge 1 - \delta_w ~\text{and}~
%	\Probop_{S_m}\[ L_Q(\Ch) \le U(\Ch, S_m, w^*, \delta_C) \] \ge 1 - \delta_C,
%}
%then the following holds with probability at least $(1 - \delta_w)(1- \delta_C)$:
%\eqa{
%L_Q(\Ch) \leq \max_{w \in \Ws(S_m, T_n, \delta_{w})} U(\Ch, S_m, w, b, \delta_C).\label{eq:ucb_worst}
%}
%\end{theorem}
\begin{theorem}
\label{thm:e2e_ps_bound}
We have
\eqa{
\Prob_{S_m\sim P^m,V\sim U^m,A}\left[L_Q(C) \leq \max_{w \in \Ws} U_{\text{RSCP}}(C, S_m, V, w, b, \delta)\right]\ge1-\delta-\delta_w.
\label{eq:ucb_worst}
}
\end{theorem}

Let $U' \coloneqq U(C, S_m, w, \delta)$, $U^* \coloneqq U(C, S_m, w^*, \delta)$ and $\Ws' \coloneqq \Ws(S_m, T_n, \delta_{w})$. Then, we have
\eqas{
\Prob_{S_m, T_n}\[ L_Q(C) \leq \max_{w \in \Ws'} U' \]
&=1 - \Prob_{S_m, T_n}\[ L_Q(C) > \max_{w \in \Ws'} U' \] \\
&\ge 1 - \Prob_{S_m, T_n}\[ \left(L_Q(C) > \max_{w \in \Ws'} U'\wedge w^* \in \Ws'\right) \vee w^* \not\in \Ws'\] \\
&\ge 1 - \Prob_{S_m}\[ L_Q(C) > \max_{w \in \Ws'} U' \wedge w^* \in \Ws' \] - \Probop_{S_m^X, T_n^X} \Big[ w^* \not\in \Ws' \Big] \\
&\ge 1 - \Prob_{S_m}\[ L_Q(C) > U^* \] - \Probop_{S_m^X, T_n^X}\Big[ w^* \not\in \Ws' \Big] \\
&\ge 1-\delta-\delta_w,
}
as claimed.


%%
%%
%%
\section{Proof of Lemma \ref{lem:mono_rejection_bound}} \label{apdx:mono_rejection_bound_proof}

%\textbf{Monotonicity in $w_i$.} 
Let $w$ and $v$ be IWs where $w(x_i) \ge v(x_i)$ and $w(x_j) = v(x_j)$ for $j \ne i$.
Additionally, we use the following shorthands:
\eqas{
n_w &\coloneqq \sum_{i=1}^m \mathbbm{1} \( U_i \le \frac{w(x_i)}{b} \), \\
T_{n_w} &\coloneqq \left\{ (x_i, y_i) \in S_m \vmid U_i \le \frac{w(x_i)}{b} \right\}, \\
k_{w} &\coloneqq \sum_{(x, y) \in T_{n_w}} \mathbbm{1} \( y \notin C(x) \), \\
n_v &\coloneqq \sum_{i=1}^m \mathbbm{1} \( U_i \le \frac{v(x_i)}{b} \), \\
T_{n_v} &\coloneqq \left\{ (x_i, y_i) \in S_m \vmid U_i \le \frac{v(x_i)}{b} \right\}, \text{~and} \\
k_{v} &\coloneqq \sum_{(x, y) \in T_{n_v}} \mathbbm{1} \( y \notin C(x) \).
}
Here, $n_w \ge n_v$ since $w(x_i) \ge v(x_i)$.
Finally, recall that $F(k; m, \theta)$ be the cumulative distribution function of a binomial random variable $\sum_{i=1}^{m} X_{i}$, where $X_i \sim \text{Bern}(\theta)$.

\textbf{Increasing case.}
If ${y_i} \notin C(x_i)$, 
there are two cases to consider: \benum
\item If $\frac{v(x_i)}{b} < U_i \le \frac{w(x_i)}{b}$, then we can verify that $n_w=n_v+1$ and $k_w=k_v+1$. 
\item Otherwise, we can verify that $n_w=n_v$ and $k_w=k_v$. 
\eenum 
In both cases, $F(k_v; n_v, \theta)\le F(k_w; n_w, \theta)$, since $U_{\text{CP}}$ is monotonically jointly increasing (more precisely, non-decreasing) in $(m, k)$  as in Lemma \ref{lem:mono_CP}. So
%$k_w \ge k_v$ since $(x_i, y_i)$ is more likely to be accepted in rejection sampling with $w$ than $v$.
%Thus, 
we have
\eqas{
U_{\text{RSCP}}(C, S_m, U, w, b, \delta)
&\coloneqq U_{\text{CP}}(\Lb_{T_{n_w}}(C) , \delta) \\
&= \inf \left\{ \theta \in [0, 1] \vmid  F(k_w; n_w, \theta) \leq \delta \right\} \cup \{1\} \\
&\ge \inf \left\{ \theta \in [0, 1] \vmid  F(k_v; n_v, \theta) \leq \delta \right\} \cup \{1\} \\
&\eqqcolon U_{\text{CP}}( \Lb_{T_{n_v}}(C), \delta) \\
&= U_{\text{RSCP}}(C, S_m, U, v, b, \delta), 
}
%where the inequality holds since $U_{\text{CP}}$ is monotonically increasing in $(m, k)$ jointly as in Lemma \ref{lem:mono_CP}. 
thus $U_{\text{RSCP}}$ is monotonically increasing  (more precisely, non-decreasing) in $w(x_i)$.

\textbf{Decreasing case.}
If ${y_i} \in C(x_i)$, $k_w = k_v$, thus
we have
\eqas{
U_{\text{RSCP}}(C, S_m, U, w, b, \delta)
&= U_{\text{CP}}(\Lb_{T_{n_w}}(C), \delta) \\
&\coloneqq \inf \left\{ \theta \in [0, 1] \vmid  F(k_w; n_w, \theta) \leq \delta \right\} \cup \{1\} \\
&\le \inf \left\{ \theta \in [0, 1] \vmid  F(k_v; n_v, \theta) \leq \delta \right\} \cup \{1\} \\
&\eqqcolon U_{\text{CP}}(\Lb_{T_{n_v}}(C), \delta) \\
&= U_{\text{RSCP}}(C, S_m, U, v, b, \delta), 
}
where the inequality holds since $U_{\text{CP}}$ is monotonically decreasing (or rather, non-increasing) in $m$ as in Lemma \ref{lem:mono_CP}; 
thus $U_{\text{RSCP}}$ is monotonically decreasing (or rather, non-increasing) in $w(x_i)$.



%%
%%
%%
\section{Proof of Theorem \ref{thm:iw_bound}} \label{apdx:thm:iw_bound_proof}

Recall that
\eqas{
	\ph_B(x) &\coloneqq \sum_{j=1}^K \mathbbm{1}\( x \in B_j\) \[ \frac{1}{m} \sum_{x' \in S_m^X} \mathbbm{1}\( x' \in B_j \) \], \\
	\qh_B(x) &\coloneqq \sum_{j=1}^K \mathbbm{1}\( x \in B_j\) \[ \frac{1}{n} \sum_{x' \in T_n^X} \mathbbm{1}\( x_i \in B_j \) \], \\
	p_B(x) &\coloneqq \sum_{j=1}^K \mathbbm{1}\( x \in B_j \) \int_{B_j} p(x')~ \mathrm{d}x', \text{~and} \\
	q_B(x) &\coloneqq \sum_{j=1}^K \mathbbm{1}\( x \in B_j \) \int_{B_j} q(x')~ \mathrm{d}x'.
}


%% p - p_K
Due to the assumption of (\ref{eq:smooth_assumption}), $| v(x) \cdot p(x) - p_K(x) |$ is bounded for any $x \in B_j$ as follows:
\eqa{
	| v(x) \cdot p(x) - p_B(x) |
	&= \left| \int_{B_j} p(x) \; \mathrm{d}x' - \int_{B_j} p(x') \; \mathrm{d}x' \right| \nonumber \\
	&= \left| \int_{B_j} p(x) - p(x') \mathrm{d}x'  \right| \nonumber \\
	&\le \int_{B_j} \left| p(x) - p(x') \right| \mathrm{d}x' \nonumber \\
%	&\le \int_{B_k} \frac{E}{|B_k|}  \mathrm{d}x' \\
%	&= \frac{E}{|B_k|}  \int_{B_k} \mathrm{d}x' \\
%	&= \frac{E}{|B_k|}  |B_k| \\
	&= E. \label{eq:p_p_K_bound}
}
Similarly, 
\eqa{
	| v(x) \cdot q(x) - q_B(x) | \le E. \label{eq:q_q_K_bound}
}

%% \ph - p_K
Observe that $m \ph(x) \sim \text{Binom}\(m, \int_{B_j} p(x') \mathrm{d}x' \)$ for any $x \in B_j$; thus $p_K$ is bounded with probability at least $1 - \delta'$ as follows due to the Clopper-Pearson interval $(\underline{\theta}, \overline{\theta})$:
\eqa{
	\underline{\theta}(m \ph(x); m, \delta') \le p_K(x) \le \overline{\theta}(m \ph(x); m, \delta'). \label{eq:p_K_ph_bound}
}
Similarly, 
\eqa{
	\underline{\theta}(n \qh(x); n, \delta') \le q_K(x) \le \overline{\theta}(n \qh(x); n, \delta'). \label{eq:q_K_qh_bound}
}

From (\ref{eq:p_p_K_bound}), (\ref{eq:q_q_K_bound}), (\ref{eq:p_K_ph_bound}), and (\ref{eq:q_K_qh_bound}), the following holds:
\eqas{
	\underline{\theta}(m \ph(x); m, \delta') - E &\le v(x) \cdot p(x) \le \overline{\theta}(m \ph(x); m, \delta') + E \text{~and} \\
	\underline{\theta}(n \qh(x); n, \delta') - E &\le v(x) \cdot q(x) \le \overline{\theta}(n \qh(x); n, \delta') + E. 
}

Therefore, for any $x \in B_j$, $w^*(x)$ is bounded as follows:
\eqas{
	\frac{\underline{\theta}(n \qh(x); n, \delta') - E}{\overline{\theta}(m \ph(x); m, \delta') + E} \le w^*(x) = \frac{q(x)}{p(x)} \le \frac{\overline{\theta}(n \qh(x); n, \delta') + E}{\underline{\theta}(m \ph(x); m, \delta') - E}.
}
Since we apply the Clopper-Pearson interval for $K$ partitions for both source and target, the claim holds due to the union bound.




\section{Discussion} 

\subsection{Justification on the Point-wise Bound in Theorem \ref{thm:cp_bound}} 
\label{apdx:disc_pointbound}

Let $T_1$ and $T_2$ be the parameter associated with $\Ch_1$ and $\Ch_2$. 
We claim that 
\eqas{
\Prob_{S_m\sim P^m}[U_{\text{CP}}(\Ch_2,S_m,\delta) \le \ep]\ge1-\delta 
\Longrightarrow
\Prob_{S_m\sim P^m}[U_{\text{CP}}(\Ch_1,S_m,\delta) \le \ep]\ge1-\delta
}
if $T_1 \le T_2$. In particular, considering that $\bar{L}_{S_m}(\Ch_1) \le \bar{L}_{S_m}(\Ch_2)$ when $T_1 \le T_2$ and $F(k-1; m, \theta) \le F(k; m, \theta)$,
we have
\eqas{
U_{\text{CP}}(\Ch_1,S_m,\delta) 
&\coloneqq \inf \left\{ \theta \in [0, 1] \vmid F(\bar{L}_{S_m}(\Ch_1); m, \theta) \leq \delta \right\}\cup\{1\} \\
&\le \inf \left\{ \theta \in [0, 1] \vmid F(\bar{L}_{S_m}(\Ch_2); m, \theta) \leq \delta \right\}\cup\{1\} \\
&\eqqcolon U_{\text{CP}}(\Ch_2,S_m,\delta).
}
Therefore, the following hold as claimed:
\eqas{
\Prob_{S_m\sim P^m}[U_{\text{CP}}(\Ch_1,S_m,\delta) \le \ep]
&\ge \Prob_{S_m\sim P^m}[U_{\text{CP}}(\Ch_2,S_m,\delta) \le \ep] \\
&\ge 1 - \delta.
}
This implies 


{\color{red}

One goal of the prediction set estimation finds the parameter $T$ associated with $\Ch$ such that the expected prediction set error is bounded by a specified value $\ep$---\ie
\eqas{
	L_P(\Ch) \le U_{\text{CP}}(\Ch, S_m, \delta) \le \ep.
}
Intuitively, all we want is to find a \emph{single} $\Ch$ that satisfies the above $\ep$-bound, thus we don't need to consider a bound that holds uniformly over a set of $\Ch$s, which needs to consider the union bound over different $\Ch$ in the set, thus leads to a more conservative bound (\eg the VC bound as shown in \citep{Park2020PAC}).
This aligns with the discussion in \citep{Park2020PAC}---\ie the ``direct'' bound of Theorem 1 in \citep{Park2020PAC} interpolates the realizable and the non-realizable settings to have a better sample complexity.
In particular, a PAC learning algorithm, which assumes the realizable setting---\ie assumes to know the set including the target hypothesis, can enjoy the $1/\ep$ sample complexity bound \citep{valiant1984theory}.



In solving the maximization of (\ref{eq:cp_iid}), one may regard this as multiple hypotheses testing by considering the $\ep$-bound for each $\Ch$ as a null hypothesis. If one null hypothesis is rejected and then one can check another null hypothesis (\ie look-elsewhere), the significance level $\delta$ needs to be properly discounted (\eg by Bonferroni correction); otherwise this issue is called ``multiple comparisons problem'' or ``look-elsewhere effect''. However, in our case, there is no dependency between null hypotheses---\ie regardless of the fact that one null hypothesis is reject or not, we search other null hypothesis until the $U_\text{CP}$ bound is close to $\ep$; thus we don't need correction on the significance level.

}




\subsection{Discussion on Maximization over $\Ws$} \label{apdx:disc_iw_uncertainty_set}

Recall that 
\eqas{
\Ws
%(S_m^X, T_n^X, \delta_w)
\coloneqq \left\{ w \in \realnum^m \mid 
\forall i\in[m] \;,\; \underline{w}_i \le w_i \le \overline{w}_i \wedge \underline{c} \le \mathbf{1}^T w \le \overline{c} \right\}.
}
We want to solve the following maximization 
\eqas{
	\max_{w \in \Ws}~ & U_{\text{RSCP}} ( \Ch, S_m, V, w, b, \delta).
}
This maximization can be converted to the following combinatorial optimization:
\eqas{
\max_{w \in \Ws}~ & U_{\text{RSCP}} ( \Ch, S_m, V, w, b, \delta) \\
= &\max_{w \in \Ws}~ \inf  \left\{ \theta \in [0, 1] \vmid F\( \sum_{i=1}^m \sigma_i \mathbbm{1}\(y_i \notin \Ch(x_i) \) ; \mathbf{1}^T \sigma, \theta \) \leq \delta \right\} \cup \Big\{1\Big\} \\
& \text{subj. to}~~ \underline{w}_i \le w_i \le \overline{w}_i, ~~\mathbf{1}^Tw \in [\underline{c}, \overline{c}], ~~\sigma_i = \mathbbm{1}\( V_i \le \frac{w_i}{b} \)  \qquad \forall x \in [m] \\
=& \max_{\sigma \in \{0, 1\}^m} ~ \inf  \left\{ \theta \in [0, 1] \vmid F\( \sum_{i=1}^m \sigma_i \mathbbm{1}\(y_i \notin \Ch(x_i) \) ; \mathbf{1}^T \sigma, \theta \) \leq \delta \right\} \cup \Big\{1\Big\} \\
&\text{subj. to} ~~ \underline{w}_i \le w_i \le \overline{w}_i, ~~\mathbf{1}^Tw \in [\underline{c}, \overline{c}], ~~ \sigma_i = \mathbbm{1}\( V_i \le \frac{w_i}{b} \) \qquad \forall x \in [m].
}



\section{Experiment Details} \label{apdx:expdetails}

\subsection{Domain Adaptation}

We use a fully-connected network (with two hidden layers where each layers has 500 neurons followed by ReLU and $0.5$-dropout) as a domain classifier by which the last hidden layer of ResNet101 forms a source-target indistinguishable feature map. 
We use this last hidden layer of the trained model as example space $\Xs$, where its dimension is 2048.
%Only for the experiment over synthetic data, we use {\color{red} a linear} model as the score function, and train it using the labeled training set. 
%% training: optimization parameter
For network training, we run SGD for 100 epochs with an initial learning rate of 0.1 decaying it by half for every 20 epochs. The domain adaptation regularizer is gradually increased as in \citep{dannGanin2016}.

\subsection{ImageNetC-13}
%% note on the definition on one epoch in DA
In training a model by domain adaptation, due to the excessive size of the target training set, we subsample the same size of the source training set from the target for each training epoch.



\section{Additional Results} \label{apdx:additionalresults}

%% two gaussian
\subsection{Synthetic Rate Shift by Two Gaussians} \label{apdx:twogaussians}
\todo
%% rate shift
\begin{figure}[th!]
%% oracle
\begin{subfigure}[b]{0.49\linewidth}
\includegraphics[width=\linewidth]{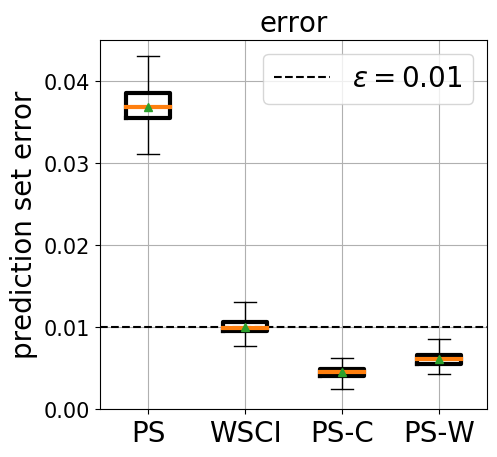}
\caption{Oracle IW \todo}
\end{subfigure}
%% estimation
\begin{subfigure}[b]{0.49\linewidth}
\includegraphics[width=\linewidth]{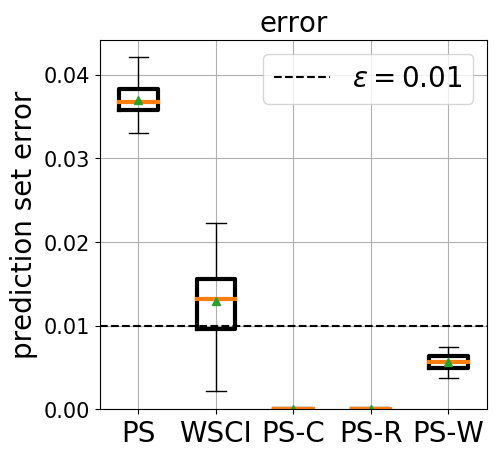}
\caption{Estimated IW \todo find another case}
\end{subfigure}
\caption{Error under the rate shift by Two Gaussians (over 100 random trials). Parameters are $m=50,000$, $\ep = 0.01$, $\delta = 0.5\times10^{-5}$, and $\delta_w=0.5\times10^{-5}$. }
\end{figure}


\textbf{Dataset.}

\textbf{With oracle IW.}

\textbf{Without oracle IW.}


\clearpage
\subsection{Prediction Set Size} \label{apdx:ps_size}

%% rate shift
\begin{figure}[h]
%% sketch
\begin{subfigure}[b]{0.49\linewidth}
\includegraphics[width=\linewidth]{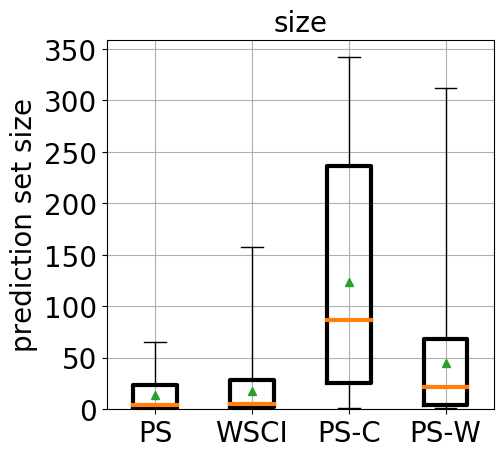}
\caption{All $\rightarrow$ Sketch}
\end{subfigure}
%% clipart
\begin{subfigure}[b]{0.49\linewidth}
\includegraphics[width=\linewidth]{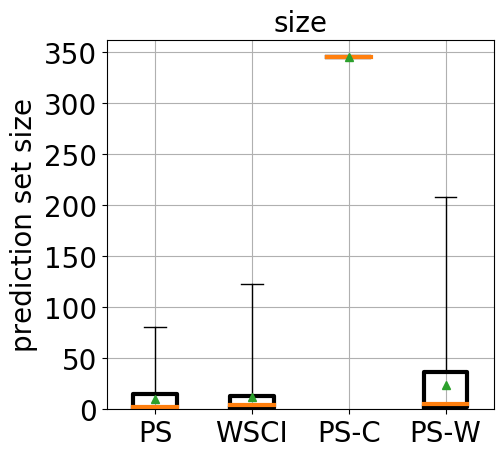}
\caption{All $\rightarrow$ Clipart}
\end{subfigure}
%% painting
\begin{subfigure}[b]{0.49\linewidth}
\includegraphics[width=\linewidth]{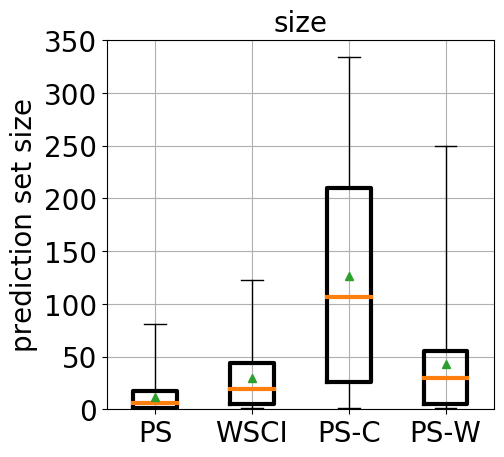}
\caption{All $\rightarrow$ Painting}
\end{subfigure}
%% quickdraw
\begin{subfigure}[b]{0.49\linewidth}
\includegraphics[width=\linewidth]{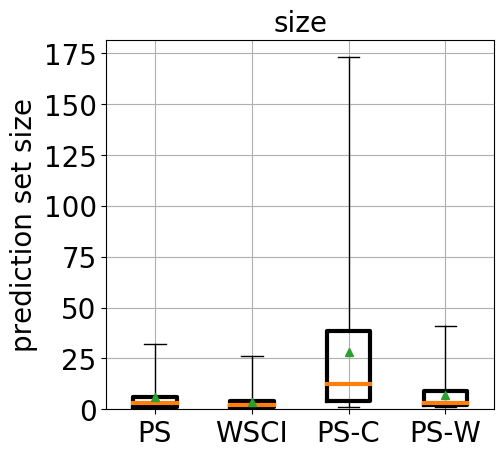}
\caption{All $\rightarrow$ Quickdraw}
\end{subfigure}
%% real
\begin{subfigure}[b]{0.49\linewidth}
\includegraphics[width=\linewidth]{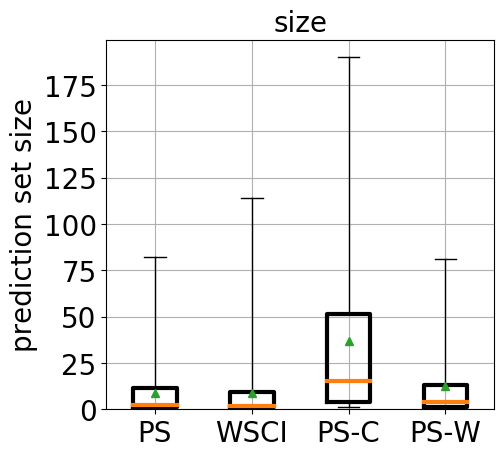}
\caption{All $\rightarrow$ Real}
\end{subfigure}
%% infograph
\begin{subfigure}[b]{0.49\linewidth}
\includegraphics[width=\linewidth]{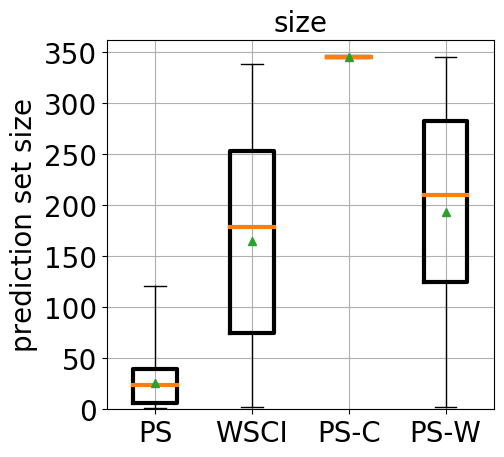}
\caption{All $\rightarrow$ Infograph}
\label{fig:domainnet:infograph}
\end{subfigure}
\caption{Size distribution under natural rate shift by DomainNet. (a-f) We consider six different natural rate shift. Parameters are $m=50,000$, $\ep = 0.1$, $\delta = 0.5\times10^{-5}$, and $\delta_w=0.5\times10^{-5}$.} 
\label{fig:domainnet}
\end{figure}

%% synthetic shift
\begin{figure}[h]
%% imagenetc
\begin{subfigure}[b]{0.49\linewidth}
\includegraphics[width=\linewidth]{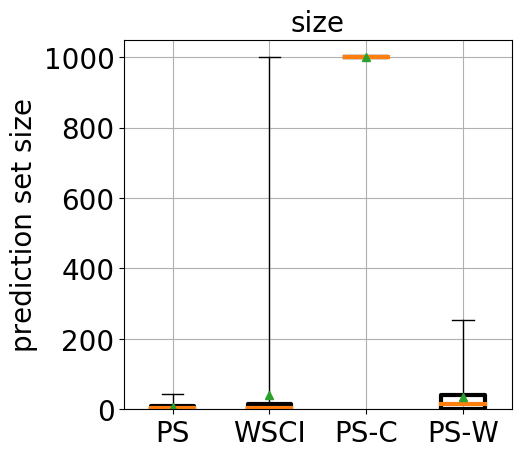}
\caption{ImageNet-C13}
\label{fig:imagenetc13}
\end{subfigure}
%% adversarial imagenet
\begin{subfigure}[b]{0.49\linewidth}
\includegraphics[width=\linewidth]{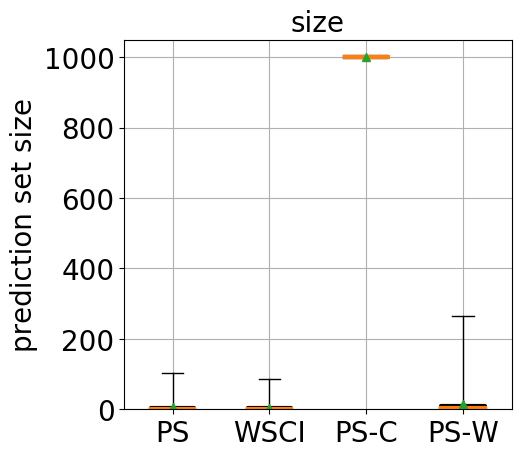}
\caption{ImageNet-PGD}
\label{fig:imagenetadvex}
\end{subfigure}
\caption{Size distribution on the shift by synthetic and adversarial perturbations on ImageNet.  Parameters are $m=20,000$, $\ep = 0.1$, $\delta = 0.5\times10^{-5}$, $\delta_w=0.5\times10^{-5}$.}
\end{figure}

\clearpage

\subsection{IW Distribution} \label{apdx:analysis_infograph}

\begin{figure}[h]
%% oracle
\begin{subfigure}[b]{0.49\linewidth}
\includegraphics[width=\linewidth]{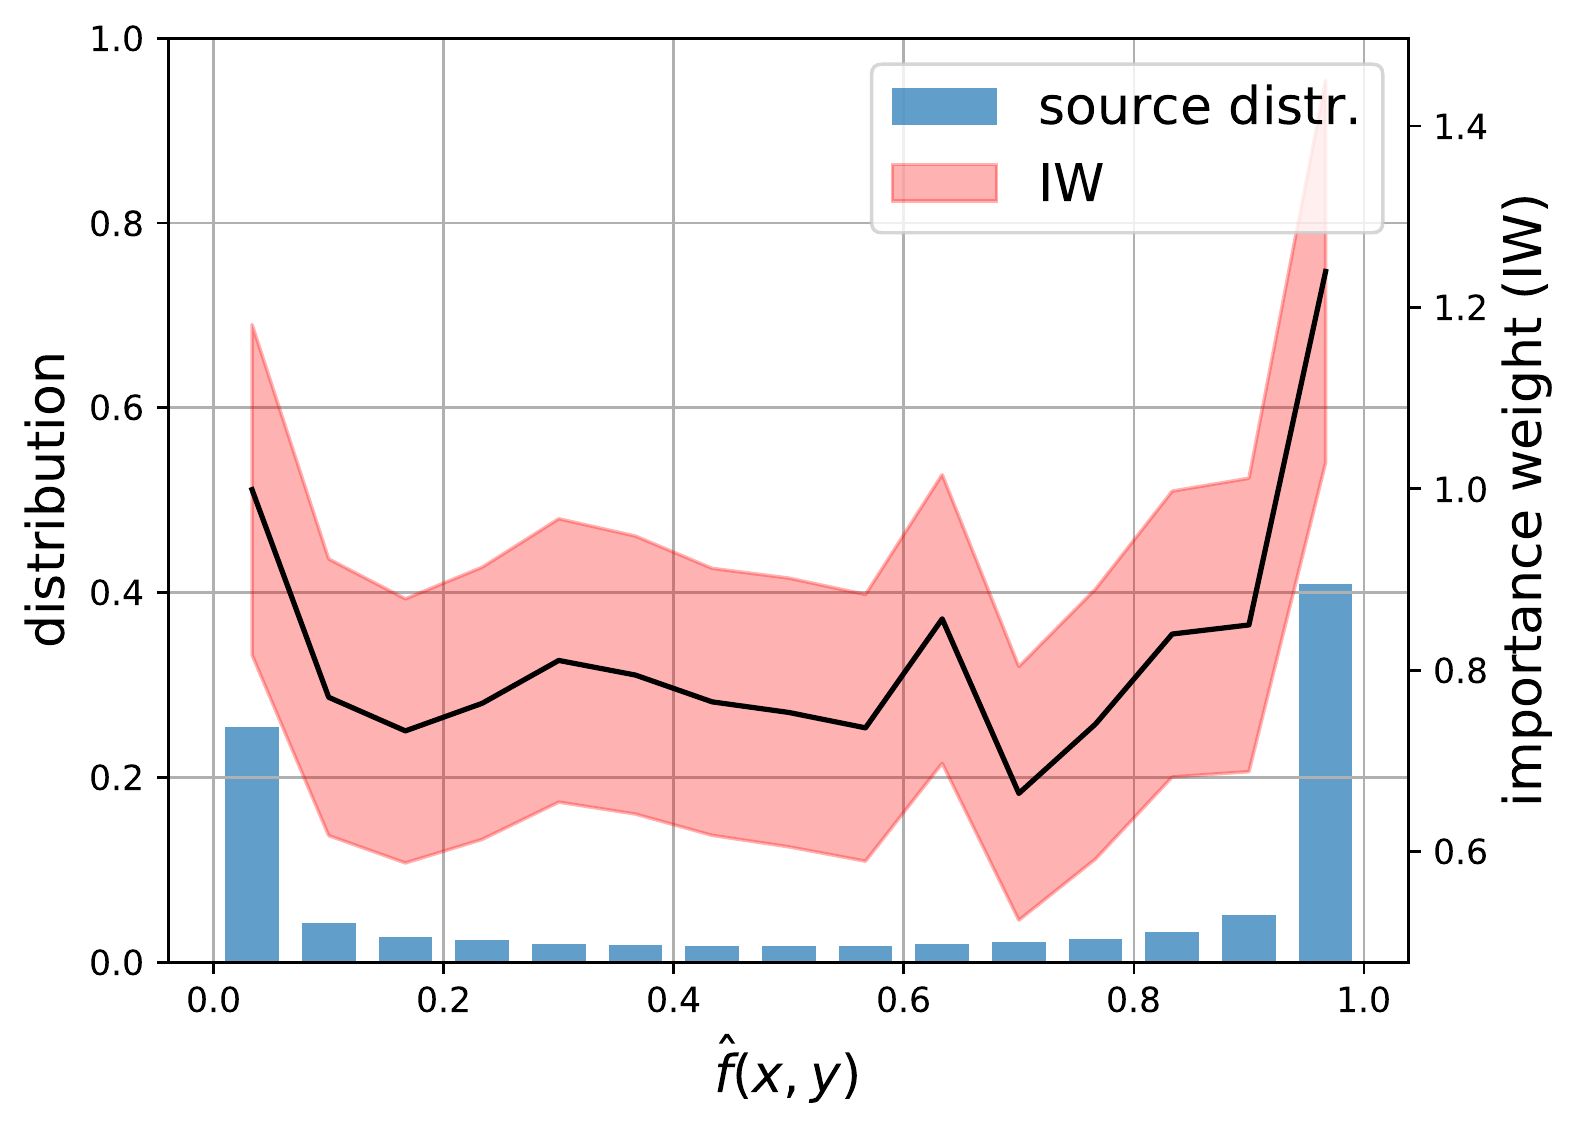}
\caption{All $\rightarrow$ Clipart}
\end{subfigure}
%% estimation
\begin{subfigure}[b]{0.49\linewidth}
\includegraphics[width=\linewidth]{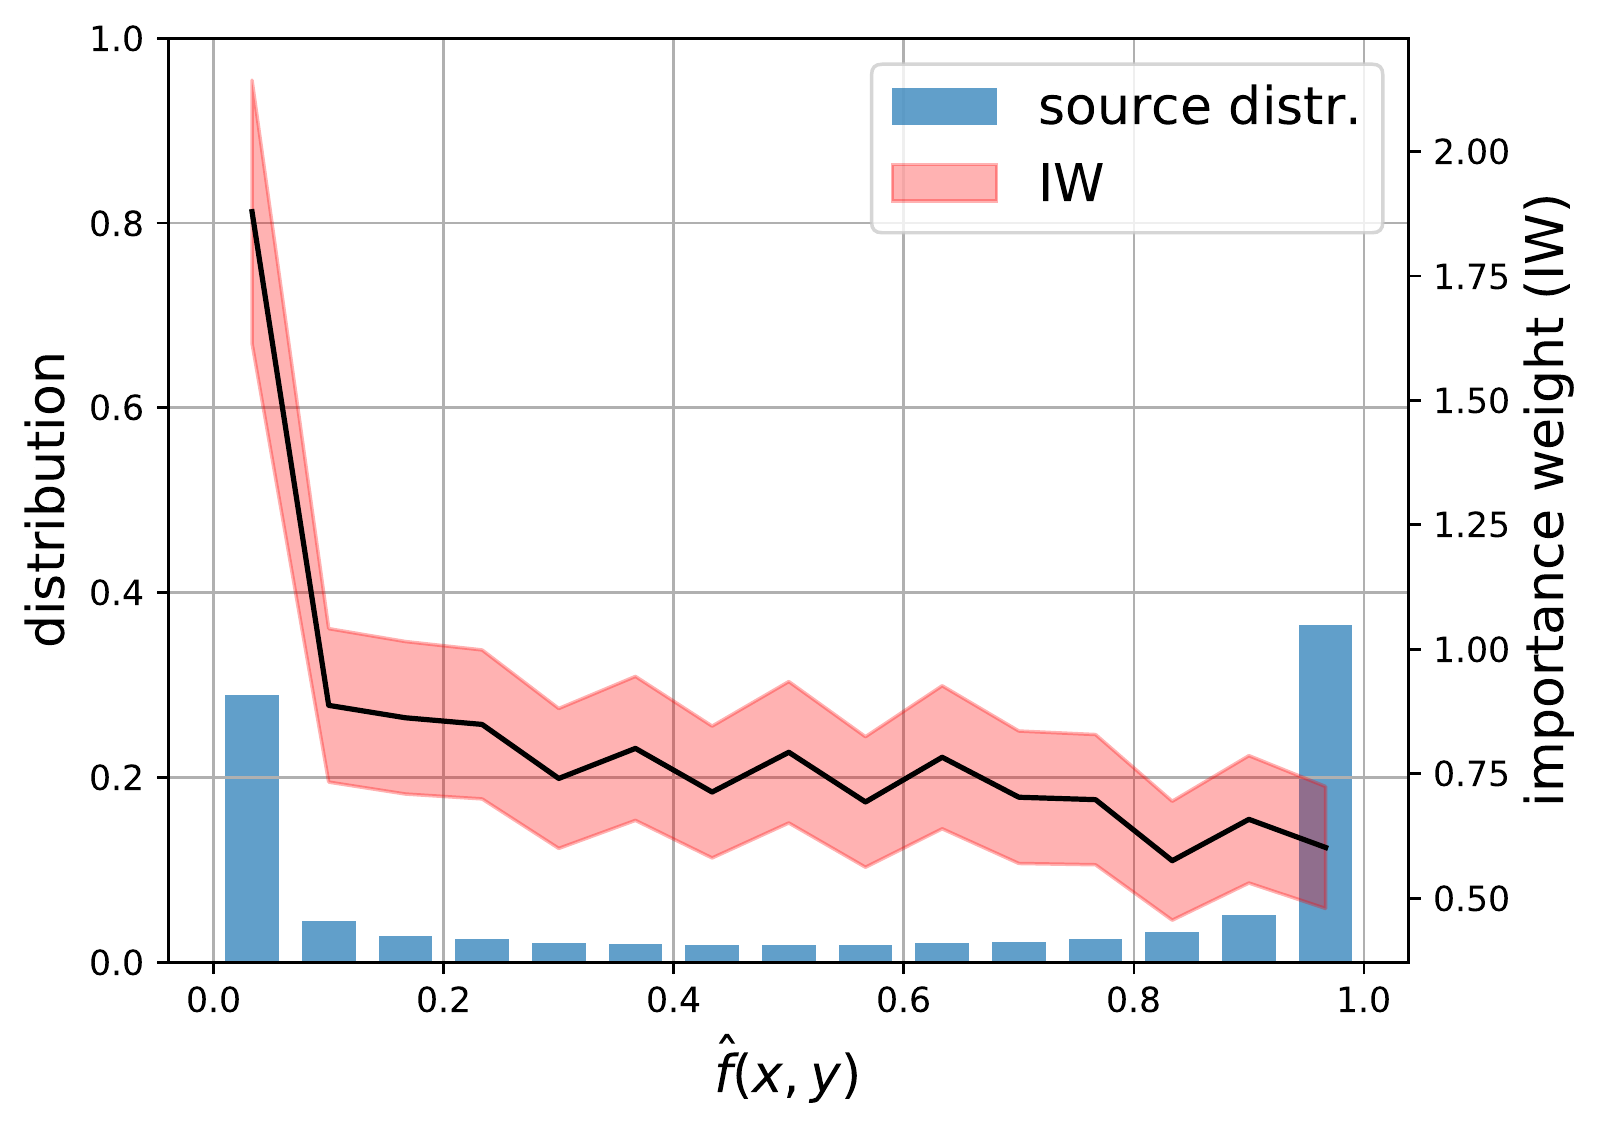}\caption{All $\rightarrow$ Infograph}
\end{subfigure}
\caption{IW distribution.\todo}
\end{figure}


\subsection{Ablation Study on Calibration} \label{apdx:ablation_imagenet}

%% sensitivity over E
\begin{figure}[h]
\centering
\begin{subfigure}[t]{0.49\linewidth}
\includegraphics[width=\linewidth]{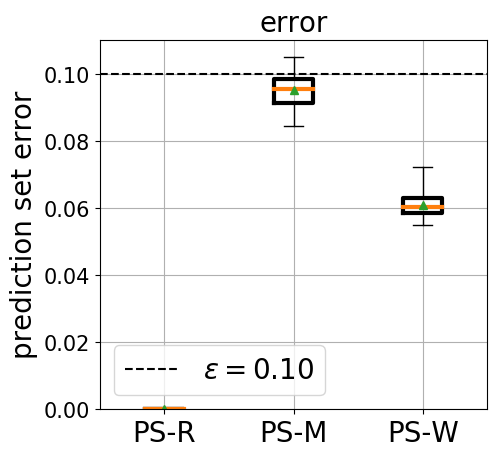}
\caption{ImageNet-C13}
\end{subfigure}
\begin{subfigure}[t]{0.49\linewidth}
\includegraphics[width=\linewidth]{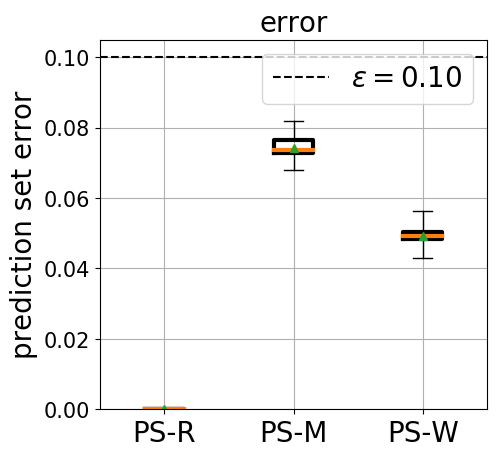}
\caption{ImageNet-PGD}
\end{subfigure}
\caption{Ablation study on calibration (over 100 random trial). Parameters are $m=20,000$, $\ep = 0.1$, $\delta = 0.5\times10^{-5}$, $\delta_w=0.5\times10^{-5}$. }
\end{figure}
